# Supplementary material for: Human-Agent Coordination in Games under Incomplete Information via Multi-Step Intent
Source: arXiv:2410.18242 source file (2025-02-17)
Supplement: Supplementary file 1 [file appendix.tex]

\begin{theorem}[Posterior Belief of Weighted Bernoulli Distribution]
\label{thm:weighted_bernoulli_posterior}
Let the prior belief about $ \theta = b(s,a) $ be modeled by a Beta distribution, $ \theta \sim \text{Beta}(\alpha, \beta) $. Using a weighted likelihood with confidence factors $c^+, c^- \in \mathbb{R}^+$ for positive evidence ($ y = 1 $) and negative evidence ($ y = 0 $), where $c^+ > c^-$, the confidence factors must satisfy condition:
\[
c^+ = \frac{\log\left(1 - (1 - \theta)^{c^-}\right)}{\log(\theta)}.
\]
Upon observing new evidence $ y $, the posterior expectation of $ \theta $ is:
\[
\mathbb{E}(\theta \mid x) = \frac{\alpha + c^+ x}{\alpha + c^+ x + \beta + c^- (1 - x)}.
\]
\end{theorem}

\begin{proof}
% Weighted Likelihood and Normalization
The weighted Bernoulli likelihood is defined as:
\[
f(x \mid \theta) = \theta^{c^+ x} (1 - \theta)^{c^- (1 - x)}, \quad x \in \{0,1\}.
\]
To ensure $ f(x \mid \theta) $ is a valid probability distribution, it must satisfy:
\[
f(0 \mid \theta) + f(1 \mid \theta) = (1 - \theta)^{c^-} + \theta^{c^+} = 1.
\]
Solving for $ c^+ $:
\[
\theta^{c^+} = 1 - (1 - \theta)^{c^-} \implies c^+ = \frac{\log\left(1 - (1 - \theta)^{c^-}\right)}{\log(\theta)}.
\]

%Bayesian Update with Beta Prior
Applying Bayes' theorem, the posterior distribution of $ \theta $ given $ x $ is proportional to the product of the likelihood and the prior:
\[
f(\theta \mid x, \alpha, \beta) \propto f(x \mid \theta) \cdot f(\theta \mid \alpha, \beta).
\]
Substituting the weighted likelihood and the Beta prior:
\begin{align*}
    f(\theta | x, \alpha, \beta) &\propto \theta^{c^+ x} (1 - \theta)^{c^- (1 - x)} \cdot \theta^{\alpha - 1} (1 - \theta)^{\beta - 1} \\
    &= \theta^{\alpha + c^+ x - 1} (1 - \theta)^{\beta + c^- (1 - x) - 1}
\end{align*}
This is the kernel of a Beta distribution with updated parameters:
\[
\theta \mid x, \alpha, \beta \sim \text{Beta}(\alpha + c^+ x, \beta + c^- (1 - x)).
\]
The posterior belief is therefore:
\[
\mathbb{E}(\theta \mid x) = \frac{\alpha + c^+ x}{\alpha + c^+ x + \beta + c^- (1 - x)}.
\]
\end{proof}
